# Supplementary material for: Exploration in two-stage recommender systems
Source: arXiv:2009.08956 source file (2020-09-01)
Supplement: Supplementary file 1 [file 06appendix.tex]

%!TEX root = ../main.tex
\section{Post- vs.\ pre-update synchronization}
\nk{Say a few words about post versus pre-update synchronization for AISTATS. Perhaps omitting the naive one in this comparison would make sense.}
